# Supplementary material for: Axial and radial axonal diffusivities from single encoding strongly diffusion-weighted MRI
Source: arXiv:2207.02526 source file (2022-07-06)
Supplement: Supplementary file 1 [file supplementary_material.pdf]

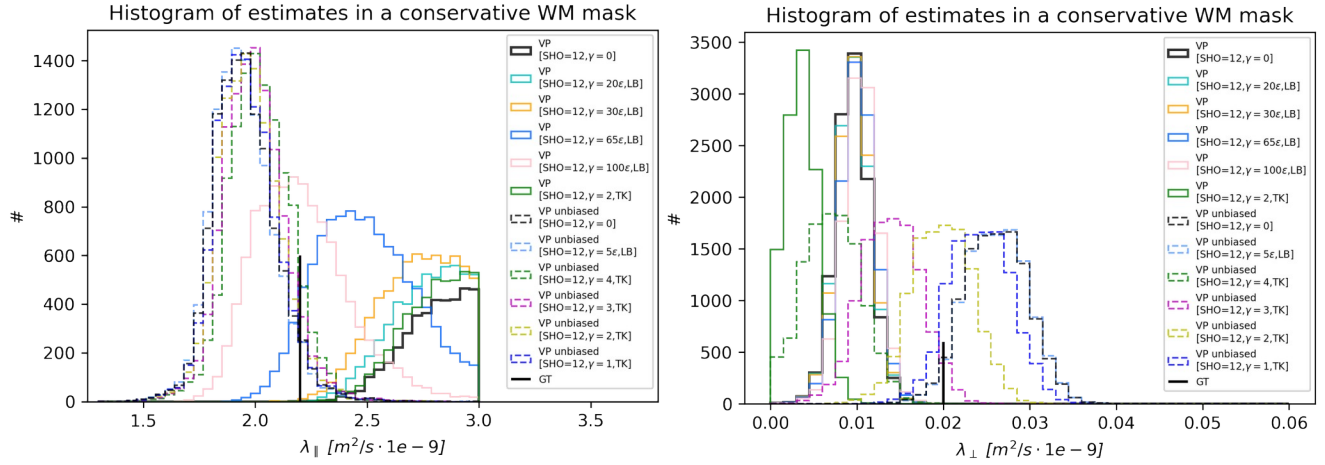

Figure S1: Histograms within the white matter region of the estimated parallel (left) and perpendicular (right) diffusivity on synthetic data after having processed the diffusion-weighted images with patch2self (after denoising) using the variable projection method (VP). Different colors and line styles correspond to different regularization amounts and types: Tikhonov (TK), Laplace Beltrami (LB); dashed lines correspond to the "unbiased" estimator (which excludes the signal' spherical mean).

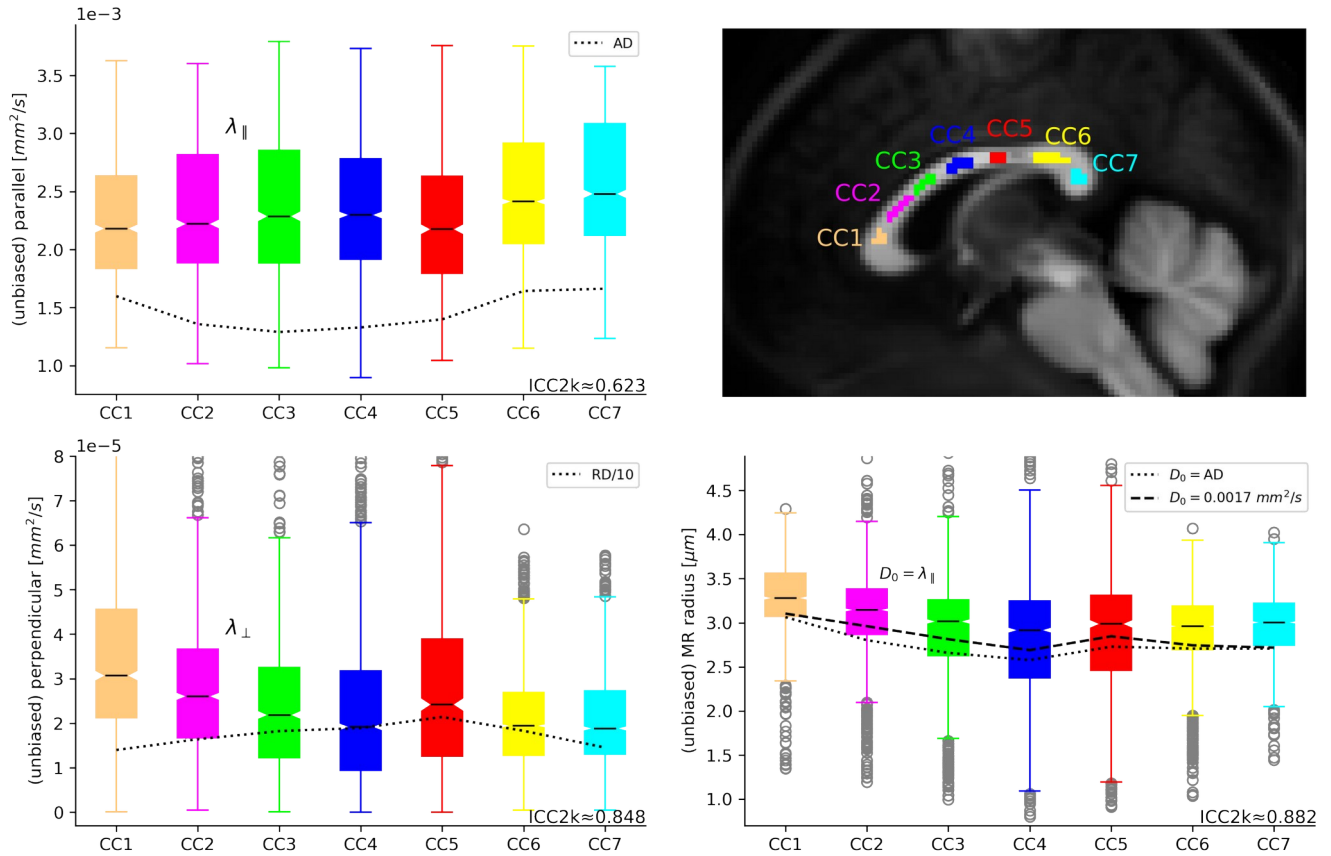

Figure S2: Distributions of estimates of parallel, perpendicular diffusivity, and MR radius in different regions of the corpus callosum considering 34 subjects of the MGH-HCP Adult Diffusion dataset. Estimates were obtained using the "unbiased" estimator based on variable projection, after the data had been post-processed with patch2self (after denoising). Intraclass correlation coefficients (2k) are reported. Values of axial (AD) and radial diffusivity (RD) - divided by 10 - from DTI are reported as well as the median values of the MR radius that would be obtained by fixing the intrinsic diffusivity to AD or by setting a specific value for it.
